# Supplementary material for: Shattered Compositionality: Counterintuitive Learning Dynamics of Transformers for Arithmetic
Source: arXiv:2601.22510 source file (2026-12-03)
Supplement: Supplementary file 1 [file To-do.tex]

\section*{For writing}

\paragraph{Tentative titles.} \YZ{Try to come up with good titles...}
\begin{itemize}
    \item Correlational matching drives learning dynamics of transformers for arithmetic tasks.
    \item Rethinking compositionality: Transformers learn to solve arithmetic tasks in unexpected ways.
    \item Rethinking compositionality: Correlational matching drives learning dynamics of transformers for arithmetic tasks.
    \item Transformers learn to build compositions for arithmetic in a reverted and shattered way
    \item Learning dynamics of transformers for arithmetic reveal reverted and shattered compositions
    \item Shattered compositionality: Transformers learn to solve arithmetic differently
    \item Shattered compositionality: the counterintuitive learning dynamics of transformers for arithmetic
    \item
    Shattered skill compositions: the counterintuitive learning dynamics of transformers for arithmetic
    \item \textbf{Shattered Compositionality: How Transformer Learning Dynamics Deviate from Human Arithmetic Composition}
    \item
    \textbf{Shattered skill compositions: the counterintuitive learning dynamics of transformers for arithmetic}
\end{itemize}

\YZ{To distinguish from existing literature, we need to emphasize learning dynamics. We are not simply prompting a model to examine compositionality, as most papers do.}

Darsh: illusion of rule learning? What are the implication for reasoning. Explain how this is relevant to actual LLMs.

\paragraph{Examples of paper writing.}
\begin{itemize}
    \item \url{https://arxiv.org/pdf/2401.09018}
    \item \url{https://arxiv.org/pdf/2008.08186}
    \item \url{https://arxiv.org/pdf/2201.11903}
\end{itemize}
