# Supplementary material for: Shattered Compositionality: Counterintuitive Learning Dynamics of Transformers for Arithmetic
Source: arXiv:2601.22510 source file (2026-12-03)
Supplement: Supplementary file 2 [file dump.tex]

\section*{Data dump from appendix}

\subsection{Four Operand Addition}

We trained the model on four operands additions, where each operand is uniformly sampled from 0 to 999.

\subsubsection{Learning Order}

In this variant, we feed the raw integers as data to the model, for both training and testing. For data format, we experimented with both plain output format and reverse output format.

For plain output format, the training data takes the form:

\begin{verbatim}
841+629+821+539=2830$
113+114+812+281=1320$
417+10+168+81=676$
\end{verbatim}

For reverse output format, the training data takes the form:
\begin{verbatim}
841+629+821+539=0382$
113+114+812+281=0231$
417+10+168+81=676$
\end{verbatim}

The result of the digit-wise error count vs iterations result is shown in Figure 1 (reversed output format) and Figure 2 (plain output format). In either case, we see that the most significant digit error drop first, followed by the hundreds-place error, then the tens-place error, and finally the units-place error. This suggests that model is not learning the same addition rules our humans use.

\begin{figure}[t]
    \centering
    \begin{subfigure}{0.48\textwidth} % Adjust width as needed
        \centering
        \includegraphics[width=\linewidth]{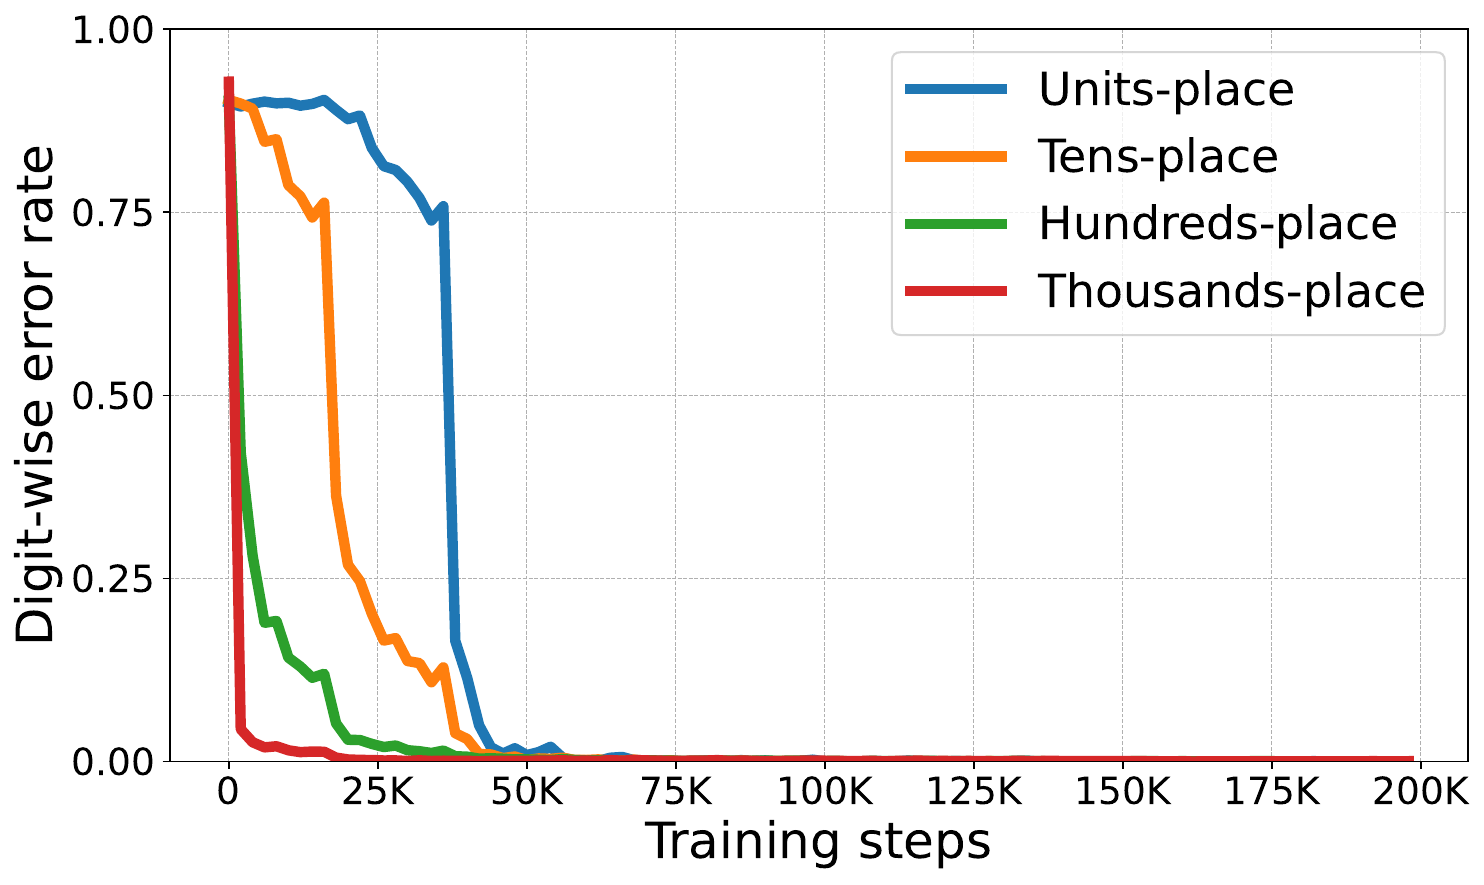} 

    \end{subfigure}%
    \hfill % Adds horizontal space between subfigures
    \begin{subfigure}{0.48\textwidth} % Adjust width as needed
        \centering
        \includegraphics[width=\linewidth]{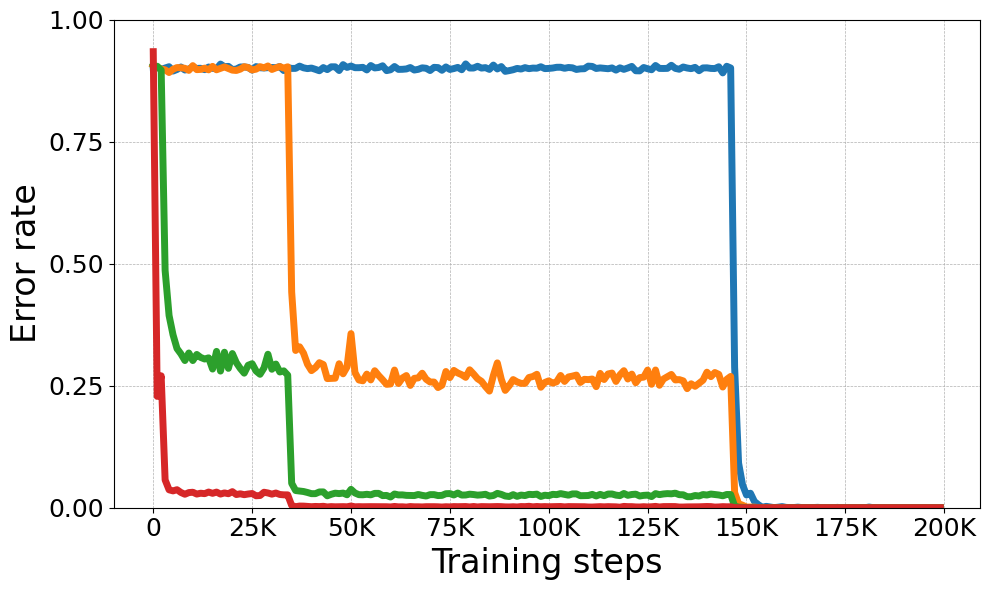} 

    \end{subfigure}
    \caption{\textbf{Transformers learn digits in the reverse order for 4-operand addition}. We train NanoGPTs and evaluate the digit-wise error rate across 200K training steps. Models learn digits from the most significant digit to the least significant digit. \textbf{Left}: 4-operand 0–999 plain output format, temperature 0.8 \eqref{eq:plain} \textbf{Right}: 4-operand 0–999 reversed output format, temperature 0.8 \eqref{eq:reverse}}
    \label{fig:10}
\end{figure}

\begin{figure}[htbp]
  \centering
  \includegraphics[
    width=0.8\linewidth,      % comma here!
    % height=0.8\textheight,    % comma here too
    keepaspectratio           % preserve aspect ratio
  ]{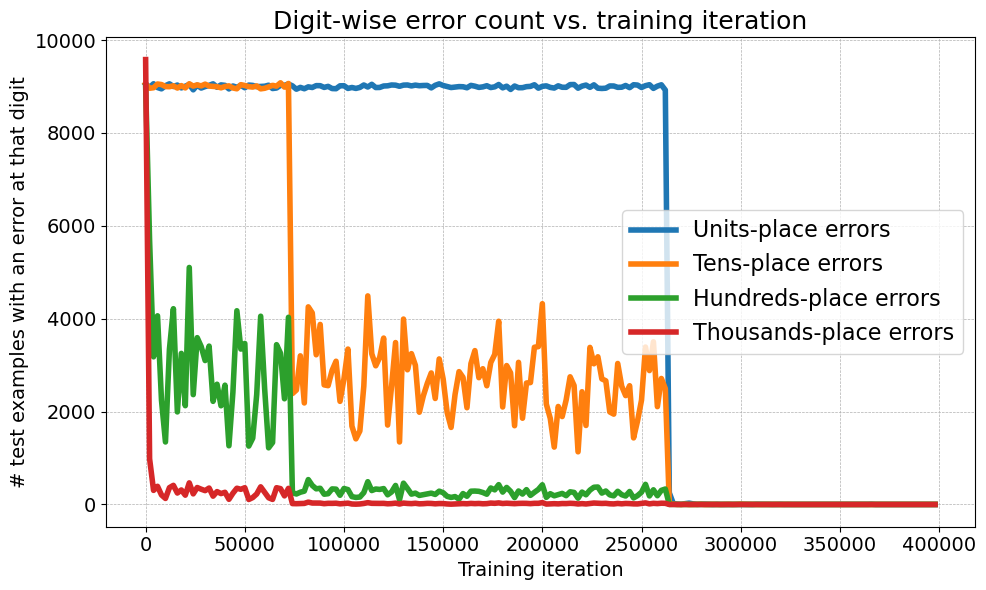}
  \caption{\textbf{Left}: 4-operand 0–999 reversed output format, temperature 0 (greedy decoding) \eqref{eq:reverse}}
  \label{fig:digit-error}
\end{figure}

The learning order is similar if we use temperature 0 (greedy decoding.)

The training accuracy and loss versus iteration is shown in Figure 3 (for reversed output format) and Figure 4 (for plain output format). Comparing the two figures, we see that the phase change in fact happened earlier in the plain output format case, while the final accuracy is higher in the reversed format case by around 1 percent (100\% vs 99\%). 

\begin{figure}[htbp]
  \centering
  \includegraphics[
    width=0.8\linewidth,      % comma here!
    % height=0.8\textheight,    % comma here too
    keepaspectratio           % preserve aspect ratio
  ]{Figures/Images/4 operand 0-999 reversed training.png}
  \caption{Training Accuracy \& Loss (4 operand 0-999 reversed output format).}
  \label{fig:digit-error}
\end{figure}

\begin{figure}[htbp]
  \centering
  \includegraphics[
    width=0.8\linewidth,      % comma here!
    % height=0.8\textheight,    % comma here too
    keepaspectratio           % preserve aspect ratio
  ]{Figures/Images/4 operand 0-999 plain training.png}
  \caption{Training Accuracy \& Loss (4 operand 0-999 plain output format).}
  \label{fig:digit-error}
\end{figure}

\subsubsection{Mutual Information Measurement}

The mutual information measurement between different pairs of digit of input-output and output-output is shown respectively in Figure 5 and Figure 6. The data used for MI measurement is structured that each input number is uniformly drawn from 100 to 999, while the examples whose result is less than 1000 are rejected. It takes the format:

$a_0a_1a_2+b_0b_1b_2+c_0c_1c_2+d_0d_1d_2=o_0o_1o_2o_3$.

Here we use the reversed output format. So for input number $a$, digit $a_0$ is the hundred-place, while for output number $o$, digit $o_3$ is the thousand-place.

For input-output mutual information measurement, NMI(0,2) stands for the normalized mutual information between the hundreds-place of the input operands and the hundreds-place of the output. NMI(1,0) stands for the normalized mutual information between the tens-place of the input operands and the units-place of the output.

For output-output mutual information measurement, NMI(0,1) stands for the normalized mutual information between the units-place and the tens-place of the output. NMI(1,2) stands for the normalized mutual information between the tens-place and the hundreds-place of the output.

Combining these results, we hypothesize that the model is exploiting the statistical dependencies among different digit-positions to learn addition. Specifically, in the beginning the model can easily notice that the hundreds-place digit of the input and the thousands-place digit of the output are highly dependent. Once it is able to predict the thousands-place digit of the output correctly, conditioned on the thousands-place digit of the output, the hundreds-place digit of the input and the hundreds-place digit of the output becomes dependent. Exploiting this dependency, the model learns to predict the hundreds-place digit of the output correctly, and so on.

\subsubsection{Ablation Experiment}

Another strong evidence supporting this argument is our ablation variant. We train the model on data without the most significant digit of the output. So the training data takes the form (for the reversed output format):

\begin{verbatim}
123+005+401+501=030$
811+856+239+313=912$
267+469+214+295=542$    
\end{verbatim}

The training result is shown in Figure 7. The model learns very poorly. Even after 800K iterations, the testing accuracy is still around 0.15\%. In comparison, when preserving the most significant digit of the output, the model can achieve almost perfect accuracy within 200K iterations.

\begin{figure}[htbp]
  \centering
  \includegraphics[
    width=0.8\linewidth,      % comma here!
    % height=0.8\textheight,    % comma here too
    keepaspectratio           % preserve aspect ratio
  ]{Figures/Images/4 operand 0-999 in-out NMI.png}
  \caption{Input-output Digit Pair Mutual Information (4 operand 0-999 reversed output format).}
  \label{fig:digit-error}
\end{figure}

\begin{figure}[htbp]
  \centering
  \includegraphics[
    width=0.8\linewidth,      % comma here!
    % height=0.8\textheight,    % comma here too
    keepaspectratio           % preserve aspect ratio
  ]{Figures/Images/4 operand 0-999 out-out NMI.png}
  \caption{Output-output Digit Pair Mutual Information (4 operand 0-999 reversed output format).}
  \label{fig:digit-error}
\end{figure}

\begin{figure}[htbp]
  \centering
  \includegraphics[
    width=0.8\linewidth,      % comma here!
    % height=0.8\textheight,    % comma here too
    keepaspectratio           % preserve aspect ratio
  ]{Figures/Images/4 operand 0-999 wo output leading digit training.png}
  \caption{Training without the most significant digit of output}
  \label{fig:digit-error}
\end{figure}

\subsection{Two Operand Addition}
We repeated some of the earlier experiments on 2-operand addition, where each operand is uniformly sampled from 0 to 999 as before. Though not as previously nicely separated, the digit-wise error lines still follow the reversed order for both plain and reversed output format.

In another variant, we removed the most significant digit of the output in the training dataset. Unlike the 4 operand counterpart, we managed to achieve perfect (or near perfect) accuracy with more training iterations. For the reversed output format, if the most significant digit of the output is preserved, the phase change happened at 1000 iterations. If the most significant digit is removed, the phase change happened at 2000 iterations. For the plain output format, if the most significant digit of the output is preserved, the phase change happened at 400 iterations. If the most significant digit is removed, the phase change happened at 1400 iterations. In addition, for the reversed output format in the ablation experiment, the units-place digit learns earlier than the tens-place digit.

\begin{figure}[htbp]
  \centering
  \includegraphics[
    width=0.8\linewidth,      % comma here!
    % height=0.8\textheight,    % comma here too
    keepaspectratio           % preserve aspect ratio
  ]{Figures/Images/2 operand 0-999 reversed format.png}
  \caption{Digit-wise error count vs. iterations (2-operand 0–999 reversed output format).}
  \label{fig:digit-error}
\end{figure}

\begin{figure}[htbp]
  \centering
  \includegraphics[
    width=0.8\linewidth,      % comma here!
    % height=0.8\textheight,    % comma here too
    keepaspectratio           % preserve aspect ratio
  ]{Figures/Images/2 operand 0-999 plain format.png}
  \caption{Digit-wise error count vs. iterations (2-operand 0–999 plain output format).}
  \label{fig:digit-error}
\end{figure}

\begin{figure}[htbp]
  \centering
  \includegraphics[
    width=0.8\linewidth,      % comma here!
    % height=0.8\textheight,    % comma here too
    keepaspectratio           % preserve aspect ratio
  ]{Figures/Images/2 operand 0-999 wo output leading digit reversed.png}
  \caption{Digit-wise error count vs. iterations (2-operand 0–999 without the most significant digit of the output, reversed output format).}
  \label{fig:digit-error}
\end{figure}

\begin{figure}[htbp]
  \centering
  \includegraphics[
    width=0.8\linewidth,      % comma here!
    % height=0.8\textheight,    % comma here too
    keepaspectratio           % preserve aspect ratio
  ]{Figures/Images/2 operand 0-999 wo output leading digit plain.png}
  \caption{Digit-wise error count vs. iterations (2-operand 0–999 without the most significant digit of the output, plain output format).}
  \label{fig:digit-error}
\end{figure}

\subsection{Comparison}

We consider the task of comparing two 4-digit numbers to understand how small transformers perform the comparison task. The comparison task can be considered as a toy setting for sorting, as the model needs to understand just the ordering between two numbers. For the experiment, we considered two numbers $a$ and $b$, and then asked the model to predict the relation ($>$, $<$, or $=$) between the numbers.

\subsubsection{Experiment 1: Skewed Dataset (\num{1000000} Samples)}

We started with a dataset of \num{1000000} random 4-digit number pairs. The model quickly learned comparisons when the most significant differing digit was at the thousands or hundreds place. However, when the most significant differing digit was at the tens place, it required about \num{50000} iterations to learn the comparison, and for numbers where the most significant differing digit was at the units place, it took around \num{200000} iterations to reach \SI{70}{\%} accuracy. The model never reliably learned to predict the equality relation. We attribute this behavior to the underlying data distribution: in the \num{1000000}-sample dataset, approximately \SI{88}{\%} of examples have different thousands digits, around \SI{10}{\%} have the same thousands digit, about \SI{1}{\%} of samples have their most significant difference at the tens place, \SI{0.01}{\%} at the units place, and only \SI{0.001}{\%} of examples have all four digits the same.

\begin{figure}[htbp]
  \centering
  \includegraphics[
    width=0.8\linewidth,
    keepaspectratio
  ]{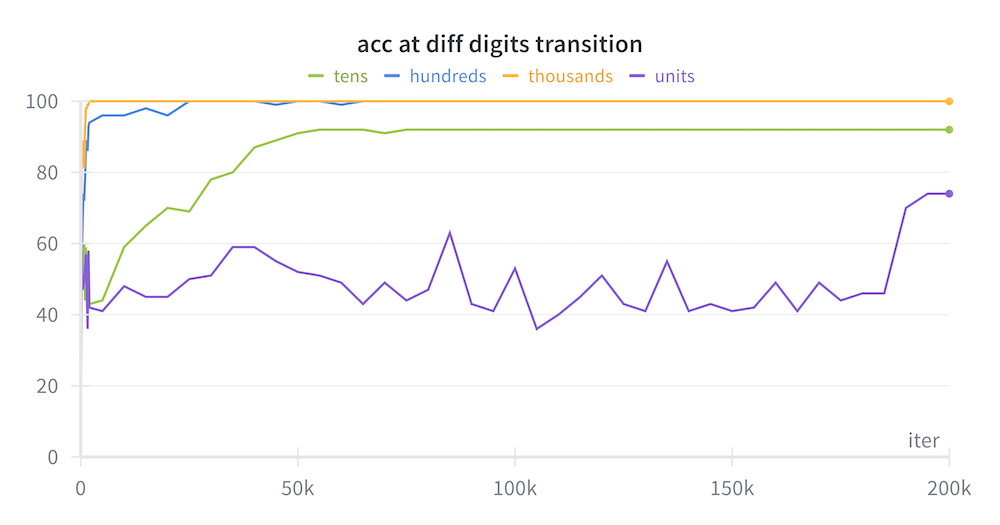}
  \caption{Accuracy comparison for 1M dataset with different significant digits.}
  \label{fig:acc-1M}
\end{figure}

\subsubsection{Experiment 2: Partially Balanced Dataset (\num{189000} Samples)}

For the next experiment, we used a partially balanced dataset of \num{189000} samples: \num{45000} examples each (\SI{23.8}{\%}) where the most significant differing digit was at the thousands, hundreds, tens, or units place, and \num{9000} examples (\SI{4.76}{\%}) where all digits were the same. Under this distribution, the model learned to handle cases with thousands, hundreds, and tens differences within just \num{400} iterations. However, despite the units category having the same number of samples as the other differing-digit categories, the model still struggled when the most significant differing digit was at the units place, as well as for the all-same (equality) cases. Both of these were only mastered by around \num{3000} iterations. This experiment proves that \textbf{data distribution matters a lot} in what we want the model to teach. If we provided a balanced dataset it was easier for the model to learn the task. We cannot conclusively say why comparison at the units place struggled, but it can be attributed to the fact that when all the first 3 digits are equal, the model has to effectively solve three interacting subtasks (thousands-, units-, and equality-based comparisons) rather than just two.

\begin{figure}[htbp]
  \centering
  \includegraphics[
    width=0.8\linewidth,
    keepaspectratio
  ]{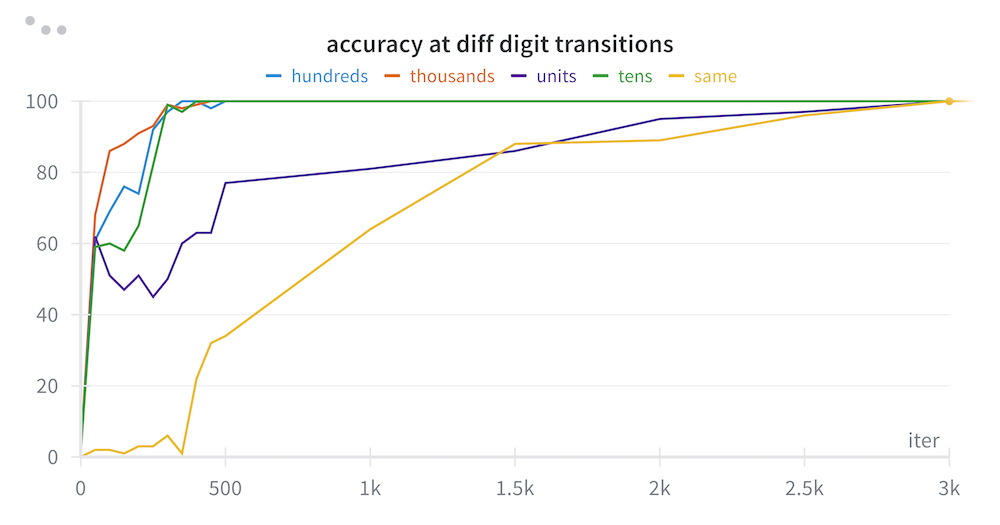}
  \caption{Accuracy comparison for 189000 dataset with different significant digits.}
  \label{fig:acc-189k}
\end{figure}

\subsection{Experiment 3: Fully Balanced Dataset (\num{45000} Samples)}

For the third setting, we used a fully balanced dataset of \num{45000} samples, with \num{9000} examples (\SI{20}{\%}) in each category: thousands-different, hundreds-different, tens-different, units-different, and all-same. In this regime, the model learned to perform the comparison task across all subtasks within about \num{1000} iterations. In the completely balanced case, the \textbf{all-same class} was learned first, and among the non-equal subtasks, the subtask where the most significant differing digit is at the \textbf{hundreds position} is learned last.

\begin{figure}[htbp]
  \centering
  \includegraphics[
    width=0.8\linewidth,
    keepaspectratio
  ]{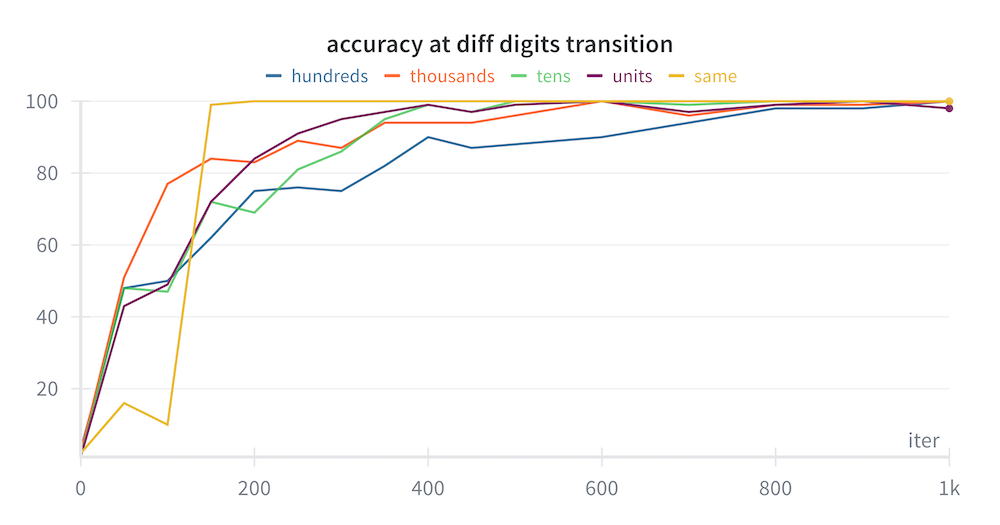}
  \caption{Accuracy comparison for 45000 dataset with different significant digits.}
  \label{fig:acc-45k}
\end{figure}

\subsection{Targeted Tests and Behavior Analysis}

Although the model reaches around \SI{80}{\%} accuracy on cases where the most significant differing digit is at the thousands or hundreds position, a targeted test reveals a gap in its behavior: when the most significant digit favors the correct answer but the remaining digits (hundreds, tens, units) are smaller, the model performs poorly until overall accuracy approaches \SI{100}{\%} (around \num{1000} iterations). This suggests that the model develops a rough sense of which numbers are larger, but still struggles with assigning the correct relative importance to different digit positions.

\begin{figure}[htbp]
  \centering
  \includegraphics[
    width=0.8\linewidth,
    keepaspectratio
  ]{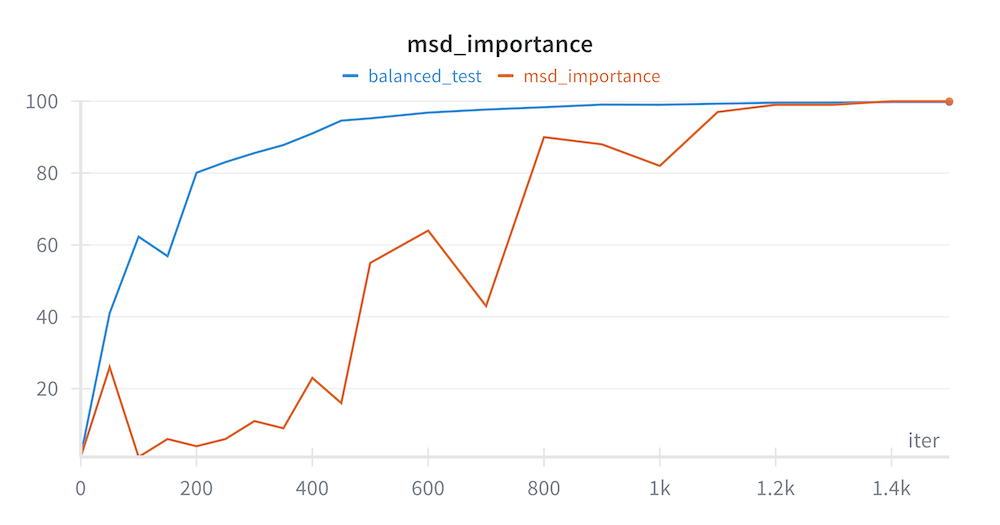}
  \caption{Comparing the importance of Most Significant Digit by creating conflict at lower positions.}
  \label{fig:msd-conflict}
\end{figure}

We tested the importance of each digit position by constructing examples where only one position was changed while the other three digits were kept identical. This produced behavior that looks quite different from human strategies. The model struggled most when we changed only the thousands digit while keeping the hundreds, tens, and units the same. It initially reached about \SI{80}{\%} accuracy on this task at around \num{200} iterations, but as training progressed and it learned to predict the equality label, it began to classify these thousands-perturbation examples as equal as well. In other words, it appeared to give more weight to the last three digits being equal than to the thousands digit being different, suggesting that different subtasks are not learned in a clean sequential manner and can interfere with each other during training.

\begin{figure}[htbp]
  \centering
  \includegraphics[
    width=0.8\linewidth,
    keepaspectratio
  ]{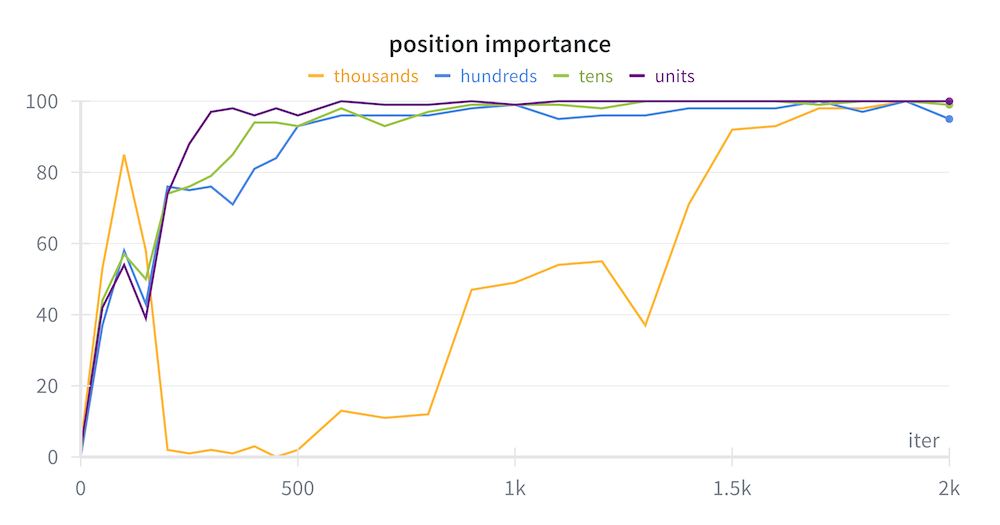}
  \caption{Accuracy when changing just one digit from the number.}
  \label{fig:position-importance}
\end{figure}

\subsection{Position Coupling}
There is a series of work that experiments with different architectural modifications and data representations, aiming to achieve better length generalization abilities. Notably, \textit{Positional Coupling} (illustrated in Figure 12, also called \textit{Abacus}) \citep{mcleish2024transformers, cho2024arithmetic} is proposed, which captures how the inherent positional information could be utilized to solve a specific task. 

\begin{figure}[htbp]
  \centering
  \includegraphics[
    width=0.8\linewidth,      % comma here!
    % height=0.8\textheight,    % comma here too
    keepaspectratio           % preserve aspect ratio
  ]{Figures/Images/abacus embedding.png}
  \caption{Visualization of Positional Coupling (Abacus Embedding).}
  \label{fig:digit-error}
\end{figure}

These works report significant length generalization improvements are observed on transformer models trained with positional coupling. One work claims that models trained with at most 20 digit operands can generalize to problems with 120 digit operands. We wonder whether models trained in such fashion would exhibit different learning mechanism, since computation pattern memorization is obviously not suitable for length generalization.

We experimented with 2 operand 0 to 9999 addition. The digit-wise error vs iterations pattern is shown in Figure 13. The difference from the result using absolute embedding is that the units-place error drops early, while the lowest three place errors roughly drop together.

Further experiment could explore what pattern will emerge if we train models learn 4 operand addition using positional coupling techniques.

\begin{figure}[htbp]
  \centering
  \includegraphics[
    width=0.8\linewidth,      % comma here!
    % height=0.8\textheight,    % comma here too
    keepaspectratio           % preserve aspect ratio
  ]{Figures/Images/2 operand 4 digit addition with abcus embedding digitwise error.png}
  \caption{Digit-wise error count vs. iterations (2-operand 0–9999 addition using positional coupling, reversed format).}
  \label{fig:digit-error}
\end{figure}

\clearpage
\subsection{Subtraction}
Using grade school arithmetic rules, performing both addition and subtraction require human beings to remember and utilize the partial result (in addition, it's "carry"; in subtraction, it's "borrow") of previous calculation when performing higher-place digit calculation. Given similar algorithmic nature of addition and subtraction, we hypothesize that transformer models are adopting the same underlying learning mechanism to approximate the final result.

We consider 2 operands subtraction task, where each operand range from 0 to 999. The result shown in Figure 14 shows similar trend, if we treat the sign digit as the most significant digit in the result.

\begin{figure}[htbp]
  \centering
  \includegraphics[
    width=0.8\linewidth,      % comma here!
    % height=0.8\textheight,    % comma here too
    keepaspectratio           % preserve aspect ratio
  ]{Figures/Images/2 operand 0-999 subtraction bd reversed format digitwise error.png}
  \caption{Digit-wise error count vs. iterations (2-operand 0–999 subtraction, reversed format).}
  \label{fig:digit-error}
\end{figure}

\subsection{Multiplication}
We are curious whether the same phenomenon occurs in other arithmetic tasks, such as multiplication. We started with 0-999 times one-digit, then went on to 0-999,999 times one-digit. 

Here we generated the training dataset to contain balanced digit length. Take the 0-999,999 times one-digit task as an example. The training data has 10,000 examples, consisting of 
all 100 1-digit * 1-digit, 
200 2-digit * 1-digit, 
400 3-digit * 1-digit examples
800 4-digit * 1-digit examples
1500 5-digit * 1-digit examples
7000 6-digit * 1-digit examples

The training data takes the form (for 0-999,999 times one-digit, reversed output format):
\begin{verbatim}
0*6=0$
678759*2=8157531$
667000*4=0008662$
6811*5=55043$
\end{verbatim}

\begin{figure}[htbp]
  \centering
  \includegraphics[
    width=0.8\linewidth,      % comma here!
    % height=0.8\textheight,    % comma here too
    keepaspectratio           % preserve aspect ratio
  ]{Figures/Images/0-999 times one-digit reversed format.png}
  \caption{Digit-wise error count vs. iterations (0-999 times one-digit reversed output format)}
  \label{fig:digit-error}
\end{figure}

\begin{figure}[htbp]
  \centering
  \includegraphics[
    width=0.8\linewidth,      % comma here!
    % height=0.8\textheight,    % comma here too
    keepaspectratio           % preserve aspect ratio
  ]{Figures/Images/0-999 times one-digit plain format.png}
  \caption{Digit-wise error count vs. iterations (0-999 times one-digit plain output format)}
  \label{fig:digit-error}
\end{figure}

\begin{figure}[htbp]
  \centering
  \includegraphics[
    width=0.8\linewidth,      % comma here!
    % height=0.8\textheight,    % comma here too
    keepaspectratio           % preserve aspect ratio
  ]{Figures/Images/0-999,999 times one-digit reversed format.png}
  \caption{Digit-wise error count vs. iterations (0-999,999 times one-digit reversed output format)}
  \label{fig:digit-error}
\end{figure}

\begin{figure}[htbp]
  \centering
  \includegraphics[
    width=0.8\linewidth,      % comma here!
    % height=0.8\textheight,    % comma here too
    keepaspectratio           % preserve aspect ratio
  ]{Figures/Images/0-999,999 times one-digit plain format.png}
  \caption{Digit-wise error count vs. iterations (0-999,999 times one-digit plain output format)}
  \label{fig:digit-error}
\end{figure}

The digit-wise error count versus iteration results are shown in Figure 15,16,17,18. Those figures are zoomed in version, so what they show is the early part of the total 5K iterations. Here we see a somewhat different trend: The errors of digit places that are on two sides (i.e. the most significant digit and the least significant digit) drop first, then followed by that of middle digit places.

We confirm the model's learning order by examining where the model gets wrong in the incorrect examples after 5K training iterations. As shown in Figure 19, we see it is indeed at the middle digit places that errors occur.

\begin{figure}[htbp]
  \centering
  \includegraphics[
    width=0.8\linewidth,      % comma here!
    % height=0.8\textheight,    % comma here too
    keepaspectratio           % preserve aspect ratio
  ]{Figures/Images/0-999,999 times one-digit plain format incorrect examples.png}
  \caption{Incorrect examples after 5K iterations in 0-999,999 times one-digit with plain output format task}
  \label{fig:digit-error}
\end{figure}
